# Supplementary material for: Specification sketching for Linear Temporal Logic
Source: arXiv:2206.06722 source file (2022-06-14)
Supplement: Supplementary file 1 [file appendix.tex]

% !TeX root = ../main.tex

\appendix

\section{A restricted version of the LTL sketch existence problem is \NP-Complete}\label{app:restricted-prob}

The exact complexity lower bound of the \existprob{} problem is open and adds to the list of open problems in the area of LTL inference (see Section~6 of~\cite{abs-2102-00876}).
However, here we show that for a restricted version of the \existprob{} in which Type-0 placeholders can only be substituted with propositions, one has $\NP$-completeness.

For introducing the \restexistprob, we use a modified definition of substitutions, which we refer to as \emph{restricted susbtitutions}. 
Precisely, a restricted substitution $s$ maps the Type-0 placeholders to propositions, that is, $s(\placeholder)\in \prop$ if $\placeholder\in\placeholderset_0$.

We, now, state the restricted version of the \sketchprob{} problem as follows: 
\begin{problem}[\restexistprob]
	Given a sketch $\sketch$ and a sample $\sample = (P,N)$, does there exist a complete restricted substitution $s$ for $\sketch$ such that $f_s(\sketch)$ is consistent with $\sample$?
\end{problem}

\begin{theorem}
	\restexistprob{} is in $\NP$
\end{theorem}

\begin{proof}
	Here we exploit the verifier-based definition of $\NP$ and show that: for every sketch $\sketch$ and sample $\sample$ if there exists a suitable complete restricted substitution, then there exists a complete restricted substitution that has ``size'' atmost $\poly(|\sample|,|\sketch|)$ and also is verifiable in time $\poly(|\sample|,|\sketch|)$.
	The size of a substitution $s$  is
	$\size{s} = \sum_{\placeholder\in\placeholderset^0} \size{s(\placeholder)}$.
	Here, since, Type-0 placeholders can only be replaced with propositions the witness, a substitution $s$, is clearly of size $\poly(|\sample|,|\sketch|)$ and verifying whether it is consistent with $\sample$ also requires time $\poly(|\sample|,|\sketch|)$.
\end{proof}

\begin{theorem}
	\restexistprob{} is \NP-Hard
\end{theorem}

\begin{proof}
		For proving \NP-hardness, we reduce $\SAT$ to the problem \restexistprob{}.
		Precisely, given a propositional formula $f$ in CNF, we construct a sample $\sample$ and a sketch $\sketch$ to reduce 
		an instance of $\SAT$ to an instance of \restexistprob{}.
		
		Let us then first formalize $f$.
		Let $\{x_1,\ldots,x_n\}$ and $\{C_1,\ldots C_m\}$ be the set of variables and clauses of $f$, respectively.
		We visualize $f$ as an $m\times n$ matrix $I_f$ that stores which variable appears in which clause. 
		Precisely, $I_f(i,j) =	1 \text{ if } x_j \in C_i; I_f(i,j) = -1 \text{ if } \neg x_j \in C_i;I_f(i,j) = 0 \text{ otherwise }$.
	
		Now, to construct the sample $\sample$, first we define the following:
		$F_{i,j} = \{p\} \text{ if } I_f = 1; F_{i,j} = \{q\} \text{ if } I_f = -1; F_{i,j} = \{p,q\} \text{ if } I_f = 0$. 
		The sample $\sample$ consists of one positive word $w_p=\{p,q\}^n\emptyset^\omega$ and negative words $w_{n_i}= F_{i,1}F_{i,2}\cdots F_{i,n}\emptyset^\omega$ for each $i\in\{0,\cdots, m\}$.
	
		The sketch we use is the following $\sketch = \placeholder_1 \wedge \lnext \placeholder_2\wedge\cdots \lnext^{i-1} \placeholder_i \cdots \wedge\lnext^{(n-1)} \placeholder_n$.
		
		Now proving the following claim completes the reduction:
		\begin{claim}
			$f$ is satisfiable if and only if there exists is a complete restricted substitution $s$ such that $f_s(\sketch)$ consistent with $\sample$.
		\end{claim}
	
		\begin{proof}
			($\Rightarrow$)
			Let $f$ be satisfiable with a satisfying assignment $v$ which maps variables of $f$ to 0 or 1.
			Based on $v$, we compute substitution $s$ as follows:
			\begin{align*}
			s(\placeholder_i) =
				\begin{cases}
					q \text{ if } v(x_i)=1\\
					p \text{ if } v(x_i)=0
				\end{cases}
			\end{align*}
			
			We now consider the formula $\varphi = s(\placeholder_1) \wedge \lnext s(\placeholder_2) \wedge \cdots \lnext^{i-1} s(\placeholder_i) \cdots\wedge \lnext^{n-1} s(\placeholder_n)$, obtained by applying $s$ to $\sketch$.
			We show that $\varphi$ is indeed consistent with $\sample$.
			
			First, observe that the positive word $w_p$ satisfies $\varphi$. This is because, $\varphi$ requires at least one of the propositions $p$ or $q$ to be true in the first $n$ positions, which is the case in $w_n$.
			
			Second, we show that none of the negative words satisfy $\varphi$ using contradiction.
			Towards contradiction, assume that $V(\varphi,w_{n_i})=1$ for a negative word $w_{n_i}$.
			In the corresponding clause $C_i$, we know that if $x_j$ appears a positive literal, then $w_{n_i}[j] = \{p\}$ and thus, for $w_{n_i}$ to satisfy $\varphi$, $\placeholder_j$ in $\sketch$ must be substituted by proposition $p$.
			This means that $v$ assigns $x_j$ to 0. 
			Consequently, $v$ assigns positive literals to 0 and similarly, it assigns negative literals to 1. 
			This results in clause $C_i$ to be false and thus, contradicts that $v$ is an satisfying assignment. 

			($\Leftarrow$) Let $s$ be a complete restricted substitutions such that $f_s(\sketch)$.
			Now, clearly, $s(\placeholder)$ will be either $p$ or $q$, since otherwise $f_s(\sketch)$ will not satisfy positive word $w_p$.
			Thus, based on $s$, we define the assignment $v$ as follows:
			\begin{align*}
			v(x_i) =
				\begin{cases}
					1 \text{ if } \placeholder_i=q\\
					0 \text{ otherwise } \placeholder_i=p
				\end{cases}
			\end{align*}
			We now show that $v$ satisfies $C_i$ for any $i\in\{1,\cdots,m\}$.
			Suppose not, then $v(x_j) = 0$ if $x_i$ appears positively in $C_i$,
			and $v(x_j) = 1$ if $x_j$ appears negatively in $C_i$. 
			This, by construction, implies that $s(\placeholder_j)=p$ if $w_{n_i}[j]=\{p\}$ and $s(\placeholder_j)=q$ if $w_{n_i}[j]=\{q\}$.
			This means $w_{n_i}$ satisfies $f_s(\sketch)$ leading to a contradiction.
		\end{proof}
\end{proof}
